# Supplementary material for: Almost all quantum channels are equidistant
Source: arXiv:1612.00401 ancillary file (2017-12-12)
Supplement: Supplementary file 1 [file supp-mat.pdf]

In[1]:=

# Supplementary material for the paper "Almost all quantum channels are equidistant"

Out[1]= Almost all quantum channels are equidistant for material paper Supplementary the

```
In[2]:= ClearAll["Global`*"];
```

In[3]:=

## The support of the SMP distribution

Out[3]= distribution of SMP support the The

```
In[4]:= uxy = 9 u^2 (x + y + 2) - 9 u (x - y) (x + y - 1) + 2 (x + y - 1) ^3;
txy = (x + y - 1) ^2 + 3 u (y - x + u);
yxy = uxy + Sqrt[uxy^2 - 4 txy^3];
densxy = Abs[(yxy^(2 / 3) - 2^(2 / 3) txy) / (2^(4 / 3) Sqrt[3] Pi u yxy^(1 / 3))];
supp = uxy^2 - 4 txy^3 // Factor
disc = Discriminant[supp / u^2, u] // FullSimplify
discsol = Solve[disc == 0, y]
yc = FullSimplify[y /. discsol[[2]], x > 0]
```

Out[8]= $-27 u^2 \left(4 - 8 u^2 + 4 u^4 - 12 x - 20 u x - 20 u^2 x - 12 u^3 x + 13 x^2 + 22 u x^2 + 13 u^2 x^2 - 6 x^3 - 6 u x^3 + x^4 - 12 y + 20 u y - 20 u^2 y + 12 u^3 y + 22 x y - 22 u^2 x y - 10 x^2 y + 10 u x^2 y + 13 y^2 - 22 u y^2 + 13 u^2 y^2 - 10 x y^2 - 10 u x y^2 - 2 x^2 y^2 - 6 y^3 + 6 u y^3 + y^4\right)$

Out[9]= $-396\,718\,580\,736\, x\, y \left(x^3 + 3 x^2 (-4 + y) + (-4 + y)^3 + 3 x (16 + y (28 + y))\right)^3$

Out[10]=

$$\Big\{\{y\to 0\},$$

$$\Big\{y\to 4-x-\frac{6\times 2^{2/3}\,x}{\left(-4\,x+x^2+\sqrt{16\,x^2+8\,x^3+x^4}\right)^{1/3}}+3\times 2^{1/3}\left(-4\,x+x^2+\sqrt{16\,x^2+8\,x^3+x^4}\right)^{1/3}\Big\},$$

$$\Big\{y\to 4-x-\frac{6\times 2^{2/3}\,x}{\left(-4\,x+x^2+\sqrt{16\,x^2+8\,x^3+x^4}\right)^{1/3}}+3\times 2^{1/3}\left(-4\,x+x^2+\sqrt{16\,x^2+8\,x^3+x^4}\right)^{1/3}\Big\},$$

$$\Big\{y\to 4-x-\frac{6\times 2^{2/3}\,x}{\left(-4\,x+x^2+\sqrt{16\,x^2+8\,x^3+x^4}\right)^{1/3}}+3\times 2^{1/3}\left(-4\,x+x^2+\sqrt{16\,x^2+8\,x^3+x^4}\right)^{1/3}\Big\},$$

$$\Big\{y\to 4-x+\frac{3\times 2^{2/3}\left(1+i\sqrt{3}\right)x}{\left(-4\,x+x^2+\sqrt{16\,x^2+8\,x^3+x^4}\right)^{1/3}}-\frac{3\left(1-i\sqrt{3}\right)\left(-4\,x+x^2+\sqrt{16\,x^2+8\,x^3+x^4}\right)^{1/3}}{2^{2/3}}\Big\},$$

$$\Big\{y\to 4-x+\frac{3\times 2^{2/3}\left(1+i\sqrt{3}\right)x}{\left(-4\,x+x^2+\sqrt{16\,x^2+8\,x^3+x^4}\right)^{1/3}}-\frac{3\left(1-i\sqrt{3}\right)\left(-4\,x+x^2+\sqrt{16\,x^2+8\,x^3+x^4}\right)^{1/3}}{2^{2/3}}\Big\},$$

$$\Big\{y\to 4-x+\frac{3\times 2^{2/3}\left(1+i\sqrt{3}\right)x}{\left(-4\,x+x^2+\sqrt{16\,x^2+8\,x^3+x^4}\right)^{1/3}}-\frac{3\left(1-i\sqrt{3}\right)\left(-4\,x+x^2+\sqrt{16\,x^2+8\,x^3+x^4}\right)^{1/3}}{2^{2/3}}\Big\},$$

$$\Big\{y\to 4-x+\frac{3\times 2^{2/3}\left(1-i\sqrt{3}\right)x}{\left(-4\,x+x^2+\sqrt{16\,x^2+8\,x^3+x^4}\right)^{1/3}}-\frac{3\left(1+i\sqrt{3}\right)\left(-4\,x+x^2+\sqrt{16\,x^2+8\,x^3+x^4}\right)^{1/3}}{2^{2/3}}\Big\},$$

$$\Big\{y\to 4-x+\frac{3\times 2^{2/3}\left(1-i\sqrt{3}\right)x}{\left(-4\,x+x^2+\sqrt{16\,x^2+8\,x^3+x^4}\right)^{1/3}}-\frac{3\left(1+i\sqrt{3}\right)\left(-4\,x+x^2+\sqrt{16\,x^2+8\,x^3+x^4}\right)^{1/3}}{2^{2/3}}\Big\},$$

$$\Big\{y\to 4-x+\frac{3\times 2^{2/3}\left(1-i\sqrt{3}\right)x}{\left(-4\,x+x^2+\sqrt{16\,x^2+8\,x^3+x^4}\right)^{1/3}}-\frac{3\left(1+i\sqrt{3}\right)\left(-4\,x+x^2+\sqrt{16\,x^2+8\,x^3+x^4}\right)^{1/3}}{2^{2/3}}\Big\}\Big\}$$

Out[11]= $4-6\times 2^{1/3}\,x^{1/3}+3\times 2^{2/3}\,x^{2/3}-x$

In[12]:=
# Weingarten calculus

Out[12]= calculus Weingarten

In[13]:=
```
cycles[x_] := Module[{},
    Length[PermutationCycles[x, Identity]]
   ];
length[x_] := Module[{},
    Length[x] - cycles[x]
   ];
Wg[x_] := Module[{k, l, i, w, y},
    y = PermutationCycles[x, Identity];
    k = Length[y];
    l = ConstantArray[0, k];
    For[i = 1, i ≤ k, i++,
     l[[i]] = Length[y[[i]]];
    ];
    l = Sort[l, Greater];
    w = 0;
    If[l == {1}, w = 1 / WG];
    If[l == {1, 1}, w = 1 / (WG^2 - 1)];
    If[l == {2}, w = -1 / (WG * (WG^2 - 1))];
    If[l == {3}, w = 2 / ((WG - 2) * (WG - 1) * WG * (WG + 1) * (WG + 2))];
    If[l == {2, 1}, w = -1 / ((WG - 2) * (WG - 1) * (WG + 1) * (WG + 2))];
    If[l == {1, 1, 1}, w = (WG^2 - 2) / ((WG - 2) * (WG - 1) * WG * (WG + 1) * (WG + 2))];
    If[l == {4}, w = -5 / ((WG - 3) * (WG - 2) * (WG - 1) * WG * (WG + 1) * (WG + 2) * (WG + 3))];
    If[l == {3, 1}, w =
      (2 * WG^2 - 3) / ((WG - 3) * (WG - 2) * (WG - 1) * WG^2 * (WG + 1) * (WG + 2) * (WG + 3))];
    If[l == {2, 2}, w = (WG^2 + 6) / ((WG - 3) * (WG - 2) * (WG - 1) *
          WG^2 * (WG + 1) * (WG + 2) * (WG + 3))];
    If[l == {2, 1, 1}, w = -1 / ((WG - 3) * (WG - 1) * WG * (WG + 1) * (WG + 3))];
    If[l == {1, 1, 1, 1}, w = (WG^4 - 8 * WG^2 + 6) /
       ((WG - 3) * (WG - 2) * (WG - 1) * WG^2 * (WG + 1) * (WG + 2) * (WG + 3))];
    w
   ];
expectationWg[g1_, g2_] :=
   Module[{p, perm, g1inv, g2inv, f, ia, ib, a, b, termab, termmatrix, c, i},
    p = Length[g1];
    perm = Permutations[Range[p]];
    g1inv = InversePermutation[g1];
    g2inv = InversePermutation[g2];
    f = 0;
    For[ia = 1, ia ≤ Factorial[p], ia++,
     For[ib = 1, ib ≤ Factorial[p], ib++,
       a = perm[[ia]];
       b = perm[[ib]];
       termab = d1^cycles[PermutationProduct[g1inv, a]] *
         d2^cycles[PermutationProduct[g2inv, a]];
       termab = termab * Wg[PermutationProduct[InversePermutation[a], b]] /.
         {WG → d1 * d2};
```

```
      termmatrix = 1;
      c = PermutationCycles[b, Identity];
      (*Print[c];*)
      For[i = 1, i ≤ Length[c], i++,
       (*Print[c[[i]]];*)
       termmatrix = termmatrix * (d1 * d2) * m[Length[c[[i]]]];
       (*Print[m[Length[c[[i]]]]];*)
      ];
      f = f + termab * termmatrix;
      (*Print[termab];
      Print[termmatrix];
      Print["--------------"];*)
     ]
    ];
    f
   ];
expMomentPQ[p_] := Module[{g1, g2, i, j, s},
   g1 = ConstantArray[0, Total[p]];
   g2 = ConstantArray[0, Total[p]];
   For[i = 1, i ≤ Length[p], i++,
    For[j = 1, j ≤ p[[i]], j++,
     s = Sum[p[[k]], {k, 1, i - 1}];
     g1[[s + j]] = s + j - 1 + If[j == 1, p[[i]], 0];
     g2[[s + j]] = s + j;
    ]];
   (*Print["g1=",g1];
   Print["g2=",g2];*)
   expectationWg[g1, g2] * d1^(-Length[p]) * d2^(-Total[p]) // Expand
  ];
```

In[18]:=

```
expMomentPQ[{1}]
expMomentPQ[{2}] - expMomentPQ[{1, 1}] // FullSimplify
varv = expMomentPQ[{2, 2}] - 2 * expMomentPQ[{2, 1, 1}] +
   expMomentPQ[{1, 1, 1, 1}] - (expMomentPQ[{2}] - expMomentPQ[{1, 1}])^2;
varv // FullSimplify
```

Out[18]= m[1]

Out[19]=

$$-\frac{\left(-1+d1^2\right)\left(m[1]^2-m[2]\right)}{-1+d1^2\,d2^2}$$

Out[21]=

$$\Big(2\left(-1+d1^2\right)\left(-1+d2^2\right)\Big(d1^4\,d2^4\left(m[1]^2-m[2]\right)^2+ d1^2\,d2^2\left(11\,m[1]^4-22\,m[1]^2\,m[2]-4\,m[2]^2+20\,m[1]\,m[3]-5\,m[4]\right)+ 5\left(3\,m[2]^2-4\,m[1]\,m[3]+m[4]\right)\Big)\Big)\Big/ \left(d2^2\left(-1+d1^2\,d2^2\right)^2\left(36-13\,d1^2\,d2^2+d1^4\,d2^4\right)\right)$$
